# Supplementary material for: Natural continual learning: success is a journey, not (just) a destination
Source: arXiv:2106.08085 source file (2021-12-15)
Supplement: Supplementary file 1 [file algo_bars.tex]

\begin{algorithm}[!ht]
	\DontPrintSemicolon
	\SetKw{Parameters}{parameters: }
	\SetKw{Input}{input: }
	\SetKw{Initialize}{initialize: }
																
	\Input $ \{ \{ (\b{x}_t, \b{\xi}_t) \}_{t=1}^{T_i} \}_{i=1}^{n_{\text{b}}} $, $\b{W}$, $\b{C}$ , $n ,m $
	\;
	\;
	\Initialize 
					
	$\hat{\b{h}}_t^{(i)} \leftarrow \text{zeros}(n, 1) \;\forall t, k$\;
	$\hat{\b{y}}_t^{(i)} \leftarrow \text{zeros}(m, 1)  \;\forall t, k$\;
	\;
					
	\% Sample targets from the model\;
	\For{$i=1 \ldots n_{\text{b}}$}{
		\For{$t=1 \ldots T_i$}{
			$\b{h}_t = \b{W} [\b{r}_{t-1};  \b{x}_t^{(i)}]$\;
			$\b{r}_t = \phi (\b{h}_t + \b{\xi}_t^{(i)})$\;
			$\b{y}_t^{(i)} \sim p(\b{y}_t | \b{C} \b{r}_t)$
			\tcp*{sample from observation model}
		}
	}
				
	\% Compute adjoints \;
	\For{$i=1 \ldots n_{\text{b}}$}{
		\For{$t=1 \ldots T_i$}{
			$\b{h}_t = \b{W} [\b{r}_{t-1};  \b{x}_t^{(i)}] + \hat{\b{h}}_t^{(i)}$\;
			$\b{r}_t = \phi (\b{h}_t + \b{\xi}_t^{(i)})$\;
			$\ell_t^{(i)} = \log p(\b{y}_t^{(i)} | \b{C} \b{r}_t + \hat{\b{y}}_t^{(i)})$
			\;
		}
	}
	$\ell = \sum_{i=1}^{n_{\text{b}}}\sum_{t=1}^{T_i} \ell_t^{(i)} / n_{\text{b}}$\;
	\% Compute adjoints of $\hat{\b{h}}_t^{(i)}$ and $\hat{\b{y}}_t^{(i)}$ with respect to $\ell$ via automatic differentiation
	\;
	$\overline{\b{h}}_t^{(i)} \leftarrow \text{adjoint of }\hat{\b{h}}_t^{(i)}, \quad 
	\overline{\b{y}}_t^{(i)} \leftarrow \text{adjoint of }\hat{\b{y}}_t^{(i)}$\; 
	
	$\mathbb{E} 
	\left [ \overline{\b{h}} \, \overline{\b{h}}^\top \right ]
	\approx
	\sum_{i=1}^{n_{\text{b}}} 
	\sum_{t=1}^{T_i} 
	\overline{\b{h}}_t^{(i)} (\overline{\b{h}}_t^{(i)})^\top / (n_{\text{b}} \, \mathbb{E} \left [ T \right ])$ \; 
	
	$\mathbb{E}
	\left [ \overline{\b{y}} \, \overline{\b{y}}^\top \right ]
	\approx
	\sum_{i=1}^{n_{\text{b}}} 
	\sum_{t=1}^{T_i} 
	\overline{\b{y}}_t^{(i)} (\overline{\b{y}}_t^{(i)})^\top / (n_{\text{b}} \, \mathbb{E} \left [ T \right ])$\;

	\caption{Estimating $\mathbb{E} \left[ \overline{\b{h}} \, \overline{\b{h}}^\top \right] , \mathbb{E} \left [ \overline{\b{y}} \, \overline{\b{y}}^\top \right ]$}
	\label{alg:ncl_estimate_hbar}
\end{algorithm}
